# Supplementary material for: SaPHyRa: A Learning Theory Approach to Ranking Nodes in Large Networks
Source: arXiv:2203.01746 source file (2022-03-03)
Supplement: Supplementary file 1 [file appendix.tex]

% !TEX root = main.tex
\subsection{Proof of Lemma \ref{le:SSP}}
\begin{proof}	
	Consider a hypothesis $\sh_i \in \sH$ ($i \in [k]$), we have 
	\begin{align*}
	\risk(h_i) &= \sum_{\sx \in \sX}  \Pr_{\sx_0 \sim {\dis}}[x_0=x]\loss\left(\sh(x),\lf(x)\right)\\
	&= \sum_{\sx \in \hat{\sX}} \Pr_{\sx_0 \sim {\dis}}[x_0=x]\loss\left(\sh(x),\lf(x)\right)  \\ 
	& \quad \quad + \weighte \sum_{\sx \in \tilde{\sX}} \Pr_{\sx_0 \sim \tilde{\dis}}[x_0=x]\loss\left(\sh(x),\lf(x)\right)\\
	%	&= \hat{\erisk}_i + \weighte\left(\sum_{\sx \in \tilde{\sX}} \left(\loss\left(\sh(x),\lf(x)\right)\tilde{\sD}(x)\right)\right)\\
	&= \hat{\erisk}_i +  \weighte{\riskest(h_i)}
	%	\sD(\{\sx \in \sX: \sh(\sx) \ne \lf(\sx)\}) \\
	%	&= \sD(\{\sx \in \hat{\sX}: \sh(\sx) \ne \lf(\sx)\}) + \sD(\{\sx \in \tilde{\sX}: \sh(\sx) \ne \lf(\sx)\})\\
	%	&=  \hat{\erisk}_i +	\frac{\tilde{\sD}(\{\sx \in \tilde{\sX}: \sh(\sx) \ne \lf(\sx)\})}{\weighte}\\			 
	%		&= \hat{\erisk}_i +  \frac{\risk_{\tilde{\Omega},\lf}(h_i)}{\weighte}
	\end{align*}
	%		Recall that $\tilde{\eRisk} = (\tilde{\erisk}_1,\tilde{\erisk}_2,\cdots,\tilde{\erisk}_n)$ is an $(\epsilon',\delta)$-estimation  of $\risk_{\tilde{\sD},\lf}$. Thus, with probability at least $1- \delta$, $\forall h_i \in \sH$,
	%		\begin{equation}
	%		|\risk_{\tilde{\sD},\lf}(h_i) - \tilde{\erisk}_i| \leq \epsilon'
	%		\end{equation}
	%		Hence, with probability at least $ 1 - \delta$, $\forall h_i \in \sH$
	%	We have 
	%	\begin{align*}
	%	&\Pr \left[\forall i \in [k], |\risk-\erisk_i| < \epsilon\right] \\
	%	= & \Pr \left[\forall i \in [k], |\hat{\erisk}_i +  \weighte{\riskest(h_i)}- \hat{\erisk}_i - \weighte{\tilde{\erisk}_i}| < \epsilon\right] \\
	%	= & \Pr \left[\forall i \in [k], |  \weighte(\riskest(h_i)- \tilde{\erisk}_i )| < \epsilon\right] \\
	%	=& \Pr \left[\forall i \in [k], |  {\riskest(h_i)- \tilde{\erisk}_i }| < \epsilon'\right] \ge 1 -\delta
	%	%		|\risk_{{\sD},\lf}(h_i) - \erisk_i| &= |\hat{\erisk}_i +  \frac{\risk_{\tilde{\sD},\lf}(h_i)}{\weighte} - (\hat{\erisk}_i +   \tilde{\erisk}_i) / \weighte| \\ 
	%	%		&= |\frac{\risk_{\tilde{\sD},\lf}(h_i)}{\weighte} -  \tilde{\erisk}_i) / \weighte| \\
	%	%		&\le \epsilon' / \weighte = \epsilon
	%	\end{align*}
	%		Thus, $T$ is an $(\epsilon,\delta)-$ approximation of $(H,\sX)$
\end{proof}

\subsection{Proof of Lemma \ref{lemma:vc}}
\begin{proof}
	We prove the lemma by contradiction. Assume $VC(\sH) = w > \lfloor \log(\pi_{\max} ) \rfloor + 1$. In other words, there exists a set $S = \{x_1,\cdots,x_w\} \subseteq  \sX$ that is shattered by $\sH$. 
	Recall that, for any sample $x$, the number of hypotheses in $\sH$ that outputs $1$ is at most $\pi_{\max}$. Thus, for any $i \in [w]$, we have
	\begin{align*}
	&|\{(h(x_1),\cdots,h(p_x)): h\in \sH, h(p_i) = 1\}| &\le \pi_{\max} < 2^{w-1}\\
	\Rightarrow & |\sH_S| = |\{(h(p_1),\cdots,h(p_w)): h\in \sH\}| &< 2^{w} \quad 
	\end{align*}	
	
	This contradict with the assumption that $\sH$ shatters $S$ ($|\sH_S| = 2^w$). 
\end{proof}

\subsection{Proof of Theorem \ref{LEMMA:SSP}}
\begin{proof}
	%	[Proof of theorem \ref{LEMMA:SSP}]
	We first prove that $(\tilde{\eRisk}_1,\cdots,\tilde{\eRisk}_k)$ is an $(\epsilon',\delta)$-estimation of the expected risk on estimation subspace $\tilde{\sX}$, i.e., 
	\begin{equation}
	\Pr \left[\forall i \in [k], |\riskest(h_i)-\tilde{\erisk}_i| < \epsilon'\right] \ge 1-\delta
	\label{eq:app-erisk}
	\end{equation}
	
	We consider two cases for the halt condition of Algorithm \ref{alg::ssp} as follows.

	\emph{Case 1:} The number of samples reach $N_{\max}$
	%	If the size of $X$ exceed $N_{\max}$, then, 
	In this case, base on Lemma.\ref{le:VC}, the condition in Eq. \ref{eq:app-erisk} is satisfied.
	
	\emph{Case 2:} The condition in line $10$ (	$\max_{i\in[n]}\epsilon_i \leq \epsilon'$) is satisfied.
	Consider each iteration (lines $7$-$12$) in Algorithm \ref{alg::ssp}. 
	Let $X$ be the current list of sample. 
	From on Lemma.\ref{le:Bernstein}, for each $i \in [k]$, we have
	\begin{align*}
	Pr[\riskest(h_i)-\erisk_i > \epsilon_i] \le \delta_i\\
	Pr[\erisk_i - \riskest(h_i) > \epsilon_i] \le \delta_i
	\end{align*}
	Hence, the probability of the absolute error of a hypothesis $h_i$ exceed $\epsilon_i$ is,
	\begin{align*}
	&Pr[|\riskest(h_i)-\erisk_i| \ge \epsilon_i] \\
	&\le Pr[\riskest(h_i)-\erisk_i \ge \epsilon_i] + Pr[\erisk_i - \riskest(h_i,\sX) \ge \epsilon_i] \\
	&= 2\delta_i
	\end{align*}
	Thus, in a iteration, the probability of existing a hypothesis $h_i$ that have the error exceed $\epsilon_i$ is,
	\begin{align*}
	&Pr[\exists h_i \in H: |\riskest(h_i)-\erisk_i| \ge \epsilon_i] \\
	&\le \sum_{h_i \in H} Pr[|\riskest(h_i)-\erisk_i| \ge \epsilon_i]\\
	&= \sum_{i=1}^n 2 \delta_i = \frac{\delta}{\lceil\log(\frac{N_{max}}{N_0})\rceil}
	\end{align*}
	Since we start with a collection $X$ of size $N_0$ and doubling it until the size of $X$ exceed $N_{max}$, the total number of iterations do not exceed $\lceil\log(\frac{N_{max}}{N_0})\rceil$. 
	%$C = \lceil\log(N_{max}) - \log(N_0)\rceil$. 
	Hence , for all iterations, the probability of existing a hypothesis $h_i$ that have the absolute error exceed $\epsilon_i$ is smaller than $\frac{\delta}{C} \times C = \delta$.\\
	For all iterations, with probability at least $1-\delta$,
	\begin{equation}
	|\riskest(h_i)-\erisk_i| \le \epsilon_i, \forall h_i \in H
	\end{equation}
	%	Thus, in a iteration, if $\epsilon_i \le \epsilon'$ for $\forall \epsilon_i$, $\tilde{T}$ is an $(\epsilon',\delta)-$approximation of $(H,\tilde{\sX})$.
	%In other words, we have, 
	Since the condition in line $10$ ($\max_{i\in[n]}\epsilon_i \leq \epsilon'$) is satisfied, we have 
	$$\Pr \left[\forall i \in [k], |\riskest(h_i)-\tilde{\erisk}_i| < \epsilon'\right] \ge 1-\delta$$
	Combine with Lemma.\ref{le:SSP}, we can conclude our proof.
\end{proof}

\subsection{Proof of Lemma \ref{corol:worstcase}}
\begin{proof}
	From line $13$ in algorithm \ref{alg::ssp}, the number of sample is at most 
	$$ N_{\max} = \frac{c\weighte^2}{\epsilon^2}(VC(\sH)+\ln 1/\delta).$$
	Recall that, the number of samples in the direct estimation approach is $\frac{c}{\epsilon^2}(VC(\sH)+\ln 1/\delta)$. Thus, the relative reduction in the worst-case number of samples is $1/\lambda^2$.
	%	The worst-case number of samples in the direct estimation approach is
	%	$$ \frac{c}{\epsilon^2}(VC(\sH)+\ln 1/\delta)$$
	%	The worst-case number of samples in Algorithm \ref{alg::ssp} is
	%	$$ \frac{c\weighte^2}{\epsilon^2}(VC(\sH)+\ln 1/\delta)$$
	%	Thus, the relative reduction in the worst-case number of samples is $1/\lambda^2$.
	%	\begin{equation*}
	%	\frac{\hat{N}}{N} = \alpha ^ 2.
	%	\end{equation*}
\end{proof}

\subsection{Proof of Claim \ref{claim:OUTREACH}}
	\begin{proof}
	%	See Appendix A
	We consider two cases of node $v$ as follows.
	If $v \in C_i$, $v$ can only be reached by itself.
	
	Otherwise, $v \notin C_i$. We first show that $v$ is reached by a least one node in $C_i$. 
	Consider a node $u \in C_i$. As  the graph $G$ is a connected graph, there exists a path $p$ from $u$ to $v$. Let $u'$ be the last node in $p$ that does not belong to $C_i$. Then, there exist a path from $u'$ to $v$ that does not contain any node in $C_i$. Thus, $v \in R_i(u')$.
	
	Then, we show that $v$ cannot be reached by two different node $u,w \in C_i$. We prove this statement by contradiction. Assume that $v$ is reached by both $u$ and $w$ without moving through any node in $C_i$. Consider two paths $p_1$ from $u$ to $v$ and $p_2$ from $w$ to $v$, in which $p_1,p_2$ does not contains any nodes in $C_i$. Let $v'$ be the first common nodes of $p_1$ and $p_2$. Here, we can form a circle from $u$ to $v'$, then to $w$, and finally back to $u$. Thus, $u,w,v'$ should belong to bi-component $C_i$. However, $p_1, p_2$ does not contains any node in $C_i$ (contradiction).
	%
	%		Since a node $u \in C$ can only move to a node outside of $C$ and $G$ is decomposed into a tree of bi-components, each node $v \notin C$ is reached by a cutpointin $C$. For any node $u \in C$, it only is reached by itself.\\
	%		Thus, for each node $u \in V$, it is reached by exact one node in $C$. So, every node $v \in V$ belong to an out reach set of a node in $C$
\end{proof}

\subsection{Proof of Claim \ref{claim:st}}
\begin{proof}%[Proof idea]
	Let $U'$ be the set of shortest paths $p_1 \in \sX_b$ such that $p' \in I(p_1)$ and $U''$ be the set of shortest paths $p_2 \in \sX_b$ such that $p'' \in I(p_2)$. We can show an one-to-one mapping from $U'$ to $U''$. Indeed, for each shortest path $p_1 \in U'$, we can obtain a shortest path $p_2 \in U''$ by replacing $p'$ with $p''$. 
	%	There is an one-to-one mapping from the set of shortest paths $p_1 \in \sX_b$ such that $p' \in I(p_1)$ to the set of shortest paths $p_2 \in \sX_b$ such that $p'' \in I(p_2)$ by replacing $p'$ with $p''$ in $p_2$ to obtain $p_2$. 
\end{proof}

\subsection{Proof of Lemma \ref{lemma:outreach1}}
\begin{proof}
	%	We first show that, if $p'$ is a part of $p$, then  $s \in R_i(s')$ and $t \in R_i(t')$. 
	We prove this lemma by contradiction. 
	Assume that  $s \notin R_i(s')$. We have $s \ne s'$, since $s' \in R_i(s')$. Let $u$ be the node right before $s'$ in the shortest path $p$. We have $u \notin C_i$ (since $p'$ is the maximum intra-component shortest path in $p$ that belongs to the bi-component $C_i$). Thus, $u \in R_i(s')$. Hence, all paths from $s$ to $u$ must go through $s'$ (since $s \notin R_i(s')$). This is a contradiction since $s'$ appears twice in the shortest path $p$. 
	Similarly, we can show the contradiction of assuming $t \notin R_i(t')$.
\end{proof}
\subsection{Proof of Lemma \ref{lemma:outreach2}}
\begin{proof}
	%Next, we show that, if  $s \in R_i(s')$ and $t \in R_i(t')$, then there exists an intra-component shortest path $p'$ from $s'$ to $t'$ such that $p'$ is a part of $p$. 
	We prove this statement by contradiction. From Claim \ref{claim:OUTREACH}, we have $s \notin R_i(t')$ and $t \notin R_i(s')$.
	Thus, all path from $s$ to $t$ must go through $s'$ and $t'$. The contradiction here implies that intra-component shortest path $p''$ from $s''$ to $t''$ where $(s'',t'') \in C_i$ and $(s'',t'') \ne (s',t')$.  Without loss of generality, assume $s' \ne s''$. From Lemma \ref{lemma:outreach1}, we have $s \in R_i(s'')$ (contradiction with Claim \ref{claim:OUTREACH}). 
	%Assume that $p'$ is not a part of $p$.  Thus, all path from $s$ to $t$ must go through $s'$ and $t'$. Since $p'$ is note a part of $p$, there must be a longer intra-component shortest path $p''$ from $s''$ to $t''$ where $(s'',t'') \ne (s',t')$. Without loss of generality, assume $s' \ne s''$. 
	%
	%We consider the two following cases.
	%\begin{itemize}
	%	\item $p$ does not go through the component $C_i$. In this case, there exists a circle from $s$ to $s'$ to $t'$ to $t$ and back to $s$. 
	%\end{itemize}
\end{proof}

\subsection{Proof of Lemma \ref{lemma:bca}}
\begin{proof}
First, we show that if $s \in T_i(v)$, $t \in T_j(v)$, where $i \ne j$, then $V$ is a break point of $p$.
Indeed, all shortest paths from $s$ to $t$ must pass through the bi-component $C_i$, go to $v$, and then pass through the bi-component $C_j$. Thus, $v$ must be a break point of $p$. 

Next, we show that if $i = j$, then $v$ is not a break point of $p$. 
In fact, all shortest paths from $s$ to $t$ must not pass through any bi-component $C_i'$ such that $i \ne i'$ and $v \in C_{i'}$. (Otherwise, the shortest path must go to $v$, pass through $C_{i'}$, go back to $v$. This contradict with the definition of shortest path since $v$ is visited twice.) Recall that, if $v$ is a break point of $p$, $p$ must pass through at least $w$ bi-component that $v$ belongs to (the bi-components where $v$ is source node and the target node of the intra-component shortest paths). This is contradiction since $p$ only passes through at most one bi-component that $v$ belongs to ($C_i$).
%	
%	Let $p'$ be the intra-component shortest path of $p$ in which $v$ is the source node of $p'$ and $C_i$ be the component that $p'$ belongs to. Let $t' \in C_i \setminus\{v\}$ be the target node of $p'$.
%	From Lemma \ref{lemma:outreach1}, we have $ s \in R_i(v) \setminus \{v\}$ (since $s \ne t$) and $t \in R_i(t')$. Combine with Claim \ref{claim:OUTREACH}, we have $t \notin R_i(v)$, i.e., $t \in V \setminus R_i(v)$. 
%	Let $C_i$ be the component in which $v$ is the source node of the intra-component shortest path
\end{proof}

\subsection{Proof of Lemma \ref{lemma:bcdis}}
\begin{proof}
	Recall from Lemma \ref{lemma:bc}, we have
	$$bc(v) =  {\gamma}\mathds{E}_{p \sim\dis_c}g(v,p) + bc_a(v).$$
	Thus, Eq. \ref{eq:bcdis} equivalents with the following equation 
	$$\mathds{E}_{p \sim\dis_c}g(v,p) = \eta \mathds{E}_{p \sim\dis_c^{(A)}}g(v,p).$$
	We first show that for any shortest path $p' \in \sX_c \setminus \sX_c^{(A)}$, $g_v(p')$ always returns $0$. 
	Indeed, consider a bi-component $i \notin I(A)$. For any shortest path $p'$ from $s'$ to $t'$, where $s',t' \in C_i$, all inner nodes of $p'$ belong to the bi-component $C_i$. As $A \cap C_i = \emptyset$, $v \notin C_i$. Thus, $v$ cannot be an inner node of $p'$, i.e., $g_v(p') = 0$. 
	
	Therefore, we have, 
	\begin{align*}
	\mathds{E}_{p \sim\dis_c}g(v,p) &= \sum_{p' \in \sX_c} \Pr_{p\sim\dis_c}[p=p'] g_v(p') \\
	& = \sum_{p' \in \sX_c^{(A)}} \Pr_{p\sim\dis_c}[p=p'] g_v(p') \\
	& = \sum_{p' \in \sX_c^{(A)}} \eta \Pr_{p\sim\dis_c^{(A)}}[p=p'] g_v(p') \\
	& =  \eta \mathds{E}_{p \sim\dis_c^{(A)}}g(v,p)
	\end{align*}
\end{proof}

\subsection{Proof of Lemma \ref{lemma:bcc}}
\begin{proof}
	We have 
	\begin{align*}
	\risk_c^{(A)}(\sh_v) &= \sum_{p \in \sX_c^{(A)}} \Pr_{x\sim \dis_c^{(A)}}[x=p]\loss\left(\sh_v(p),\lf_c(p)\right)\\
	&= \sum_{p \in \sX_c^{(A)}} \Pr_{x\sim \dis_c^{(A)}}[x=p]h_v(p) = \mathds{E}_{p \sim\dis_c^{(A)}}g(v,p)
	\end{align*}
	Combine with Lemma \ref{lemma:bcdis}, we have 
	$$	bc(v) = {\gamma} \eta \risk_c^{(A)}(\sh_v) + bc_a(v).$$
\end{proof}

\subsection{Pseudocode of \exactbc{} algorithm}

\begin{algorithm}[ht!]
	
	\SetKwInOut{Input}{Input}
	\SetKwInOut{Output}{Output}	
	\Input{ A decomposed graph $G$, its set of bi-components $\sC$, and a subset of nodes $A$}
	%	\Output{The sum of cutpoint  and two-hop component betweenness centrality of all nodes in $A$}
	\Output{The risks over the exact subspace $\hat{\sX}_c^{(A)}$ and the probability of the exact subspace}
	%		in the exact subspace $\hat{\sX}$ in Eq.~\ref{eq:exact-subspace}}
	$B \gets \bigcup\limits_{v \in A} Adj(v)$\\
	%		$\hat{\lambda} = 2|E| / Q$ \textcolor{gray}{ $\quad \quad \triangleright$ the number of shortest paths with length $1$}\\
	$w_t \gets 0, \forall t \in B$\\
	\For{$C_i \in \sC$}{
		\For{$s \in C_i \cap B$}{
			$\Delta_s \gets \emptyset$\\
			%		$\sigma_{st} \gets 0, \forall t \in B$\\		
			\For{$v \in Adj(s)$}{
				\For{$t \in Adj(v) \cap B$}{
					\If {$t \notin Adj(s)$}{
						%		 $\sigma_{st} \gets \sigma_{st} + 1$
						Add $t$ to $\Delta_s$\\
						$w_t \gets w_t + 1$\\
					}
				}
			}
			\For{$v \in Adj(s) \cap A$}{
				\For{$t \in Adj(v) $}{
					\If {$t \notin Adj(s)$}{
						%		$\sigma_{st}(v) \gets \sigma_{st}(v) + 1$;
						$\hat{\erisk}_v \gets\hat{\erisk}_v + \frac{1}{\gamma\eta}\frac{1}{w_t} q_{st}$\\
						%		 	\frac{\sigma_{st}(v)}{\sigma_{st}} q_{st}$\\
						$\hat{\lambda} \gets \hat{\lambda} +\hat{\erisk}_v$
					}
				}
				
				%	$\hat{\erisk}_v \gets\hat{\erisk}_v + \frac{1}{Q}\frac{\sigma_{st}(v)}{\sigma_{st}} q_{st}$\\
				%	$\hat{\lambda} \gets \hat{\lambda} +\hat{\erisk}_v$
			}
			\For{$t \in \Delta_s$}{$w_t = 0$}
		}
		%		\For{$v \in A$}{
		%		 $bc'_2(v) \gets \frac{1}{Q} BC'_2(v)$\\
		%%		 Set  $BC_a(v)$ as in Eq.~\ref{eq:bca}\\
		%%		 $t_v \gets bc_2(v) + BC_a(v)$
		%		}
		
	}
	Return $\hat{\lambda}$ and $\{\hat{\erisk}_v\}_{v \in A}$
	%	\caption{Efficient algorithm for two-hop component betweenness centrality computation}
	\caption{Algorithm \exactbc}
	\label{2hop}
	
\end{algorithm} 

Here, we present the pseudocode for the \exactbc{} algorithm.
% to efficiently compute the expected risks on the exact subspace.
First, we set $B$ as the set of all neighbors of nodes in $A$ (line 1). 
For each bi-component $C_i$, for each source node $s \in B \cap C_i$, we execute two phases as follows. In the first phase (lines 5-10), we find all the shortest paths of length $2$ from $s$ to $t \in  B \cap A$. 
Let $\Delta_s$ be the set of nodes $t$ such that the distance from $s$ to $t$ is $2$ (i.e., $d_{st} = 2$). 
For a node $t \in \Delta_s$, we denote $w_t$ as the number of shortest paths from $s$ to $t$. Initially, all we set $w_t = 0$, for all $t \in B$. To find the value of $w_t$, we iterate through all neighbors $v$ of $s$, then iterate through all neighbors $t$ of $v$. If $t$ is not a neighbor of $s$, i.e., $d_{st} = 2$, we add $t$ to $\Delta_s$ and increase the value of $w_t$ by $1$.
In the second phase (lines 11-15), we calculate the two-hop expected risks on the exact subspace of all nodes $v \in A$ based on the number of shortest paths that we found in the first phase. More precisely, for each node $v$ that is the inner node of a shortest path from $s$ to $t$, if $d_{st} = 2$, we increase the value of the expected risk $\hat{\erisk}_v$ by $\frac{1}{\gamma\eta}\frac{1}{w_t} q_{st}$.

\subsection{Proof of Lemma \ref{lemma:falsezero}}
\begin{proof}
	We prove the lemma by contradiction. Assume that $\hat{\erisk}_v = 0$, i.e., $\forall \sx \in \hat{\sX}_c^{(A)}, g_v(x) = 0$. 
	
	Recall that, $\risk_c^{(A)}(\sh_v) > 0$, i.e., there exists a shortest path $\sx \in \sX_c^{(A)}\setminus \hat{\sX}_c^{(A)}$ from $s$ to $t$, such that $g_v(x) = 1$, i.e., $v \ne s,t$ and $v \in \sx$. 
	Since $\sx \in \sX_c^{(A)}\setminus \hat{\sX}_c^{(A)}$, $len(\sx) > 2$. Let $s',t'$ be the nodes that appear before and after $v$. Let $\sx' = (s',v,t')$. 
	As $\sx'$ is a part of the shortest path $\sx$, it also is a shortest path from $s'$ to $t'$. Here, $len(\sx') = 2$, so $\sx' \in  \hat{\sX}_c^{(A)}$ (contraction since $h_v(\sx') = 1$). 
\end{proof}

\subsection{Pseudocode of \RP{} algorithm}

\begin{algorithm}[ht!]
	
	\SetKwInOut{Input}{Input}
	\SetKwInOut{Procedure}{Procedures}
	\SetKwInOut{Output}{Output}	
	\Input{A graph $G = (V,E)$, a subset of nodes $A \subseteq V$. parameters $\epsilon,\delta \in (0,1)$} 
	\Output{An rank preserving estimation of betweenness centrality of  nodes in  $A$} 
	Decompose  $G$ into bi-components $\{C_1,\ldots, C_\ell\}$\\	
	$\sX_c^{(A)},  \lf_c, \dis_c^{(A)}, H_c^{(A)}$ are defined as in Eq. \ref{eq:pisp}, Eq. \ref{eq:lf}, Eq. \ref{eq:pispdis}, Eq. \ref{eq:hypotheses}, respectively \\
	%	$\sX_c^{(A)} \gets \cup_{i=1}^{l} \left\{ s, t \in C_i | \text{all shortest paths between } s, t  \right\}$\\
	%	$\sY_c = \{0,1\}$\\
	%	Define the distribution $\dis_c^{(A)}$ as in Eq.\ref{eq:mu}\\
	$\hat{\sX}_c^{(A)} \gets \{ p \in \sX_c^{(A)} |\ len(p) = 2 \text{ and } \exists v \in A \text{ such that } g(v,p) = 1 \}$\\
	%	\{ p \in \sX_c^{(A)} |\ len(p) \leq 2 \}$\\
	$\tilde{\sX}_c^{(A)} \gets \sX_c^{(A)} \setminus \hat{\sX}_c^{(A)}$ \\
	%	 \{p \in \sX_c^{(A)} |\ len(p) > 2\}$\\
	%	Set $\hat{\sX}_c^{(A)}$ and  $\tilde{\sX}_c^{(A)}$  in Eq. \ref{eq:exact-subspace} and Eq. \ref{eq:estimation-subspace}, respectively\\ 
	%	$H_c^{(A)} \gets \{h_v\}_{v\in A}$ \\ %where $h_v$ is  is described in Eq. \ref{eq:hypothesis}\\
	Compute $\gamma, \eta$ as in Eq. \ref{eq:normalized}, Eq. \ref{eq:pnormalized}, respectively\\
	$\epsilon^* \gets \epsilon \gamma \eta$ \\
	$BS(A) \gets \max_{i=1}^\ell \left(\VD(C_i)-1,\VD(A\cap C_i) +1\right)$ \\
	%	$VC(\sH_c^{(A)}) \gets \lfloor \log(BS(A)) \rfloor + 1$\\
	%	Obtains $\{\erisk_v\}_{v\in A}$ by running \SSP{} framework in algorithm~\ref{alg::ssp} with $\sX \defeq\sX_c^{(A)} = \hat{\sX}_c^{(A)} \cup \tilde{\sX}_c^{(A)}$, $\sY \defeq \sY_c$, $\lf \defeq \lf_c$, $\sD \defeq \sD_c^{(A)}$, $\sH \defeq \sH_c^{(A)}$, algorithm \exact{} $\defeq$ \exactbc{} (see Algorithm \ref{2hop}), and algorithm \sample{} $\defeq$ \samplebc{} (see Algorithm \ref{alg::dbpath-sampling}),
	$\{\erisk_v\}_{v\in A} \gets \SSP(\sX_c^{(A)},\sD_c^{(A)},\lf_c,\sH_c^{(A)},\epsilon^*,\delta)$ with a partition $\sX_c^{(A)} = \hat{\sX}_c^{(A)} \cup \tilde{\sX}_c^{(A)}$,  algorithm \exact{} $\defeq$ \exactbc{} (see Algorithm \ref{2hop}), algorithm \sample{} $\defeq$ \samplebc{} (see Algorithm \ref{alg::dbpath-sampling}),  and $VC(\sH_c^{(A)}) = \lfloor \log(BS(A)) \rfloor + 1$\\
	%	input $\sX_c^{(A)} = \hat{\sX}_c^{(A)} \cup \tilde{\sX}_c^{(A)}$, $\sD_c^{(A)}$, $H_c^{(A)}$ and parameters $(\epsilon^*,\delta)$. Procedure \exact{} is described in Algorithm \ref{2hop}, procedure \sample{} is described in Algorithm \ref{alg::dbpath-sampling}\\
	%	, the VC dimension is computed as in Eq. \ref{eq:vc}\\
	\For{$v \in A$}{
		$bc_a\left(v\right) \gets \frac{1}{n\left(n-1\right)}\left(\sum_{C_i \in \sC| v \in C_i}\left(r_{i}\left(v\right) - 1\right)  \left(n - r_{i}\left(v\right)\right)\right)$\\
		$\tilde{bc}(v) = bc_a\left(v\right) + \gamma \eta \erisk_v$
	}
	Return $\{\tilde{bc}(v)\}_{v \in A}$
	\caption{Rank-preserving betweenness centrality (\RP{}) algorithm}
	\label{alg::RP}
	% \vspace{-0.15in}
\end{algorithm}

We now present the pseudocode for \RP{} algorithm.
At the beginning, we decompose graph $G$ into bi-components $\{C_1,\ldots, C_\ell\}$ (line 1) and compute that out reach for each node.
We define $\sX_c^{(A)},  \lf_c, \dis_c^{(A)}, H_c^{(A)}$  as in Eq. \ref{eq:pisp}, Eq. \ref{eq:lf}, Eq. \ref{eq:pispdis}, Eq. \ref{eq:hypotheses}, respectively. The sample space $\sX_c^{(A)}$ is partitioned into $\hat{\sX}_c^{(A)} \cup \tilde{\sX}_c^{(A)}$ where 
\begin{align*}
\hat{\sX}_c^{(A)} &= \{ p \in \sX_c^{(A)} |\ len(p) = 2 \text{ and } \exists v \in A \text{ s.t. } g(v,p) = 1 \} \\
\tilde{\sX}_c^{(A)} &= \sX_c^{(A)} \setminus \hat{\sX}_c^{(A)}
\end{align*}
Then, we compute  $\gamma, \eta$ as in Eq. \ref{eq:normalized}, Eq. \ref{eq:pnormalized}, respectively. The computation of $\gamma, \eta$ can be done in $O(n)$. 
Let $\epsilon^* = \epsilon \gamma \eta$. We obtain the estimation $\{\erisk_v\}_{v\in A}$ by running \SSP{} with input $(\sX_c^{(A)},\sD_c^{(A)},\lf_c,\sH_c^{(A)},\epsilon^*,\delta)$, a partition $\sX_c^{(A)} = \hat{\sX}_c^{(A)} \cup \tilde{\sX}_c^{(A)}$. In \RP algorithm, we use algorithm \exactbc{} to compute the compute the expected risks on the exact subspace, and algorithm \samplebc{} to generate a sample.

For each node $v \in V$, we compute $ bc_a\left(v\right)$ as in Eq.\ref{eq:bca} as output an estimation for the betweenness centrality 
$$\tilde{bc}(v) = bc_a\left(v\right) + \gamma \eta \erisk_v.$$

\subsection{Proof of Lemma \ref{lemma:BS}}
\begin{proof}
	Let $BS_i(A)$ be the  maximum number of nodes in $A$ that are inner nodes of a shortest path from any two nodes in a bi-component $C_i$. 
	We proving the lemma by showing that  
	$$BS_i(A) \le \min(\VD(C_i)-1,\VD(A\cap C_i) +1,|A \cap C_i|).$$
	
	Consider any shortest path $p$ from $s$ to $t$, where $s,t \in C_i$. The number of inner nodes of $p$ is $len(p) = d(s,t) \le \VD(C_i)$. Thus, we have 
	$$BS_i(A) \le \VD(C_i)-1.$$
	
	Let $u$ be the first node in $A$ and $v$ be the last node in $A$  on the shortest path $p$. As all nodes before $u$ and after $v$ do not belong to $A$, the number of inner nodes of $p$ that belong to $A$ is at most $d(u,v) + 1 \le \VD(A\cap C_i) +1$. Thus, we have,
	$$BS_i(A) \le \VD(A\cap C_i) +1.$$
	
	As all inner nodes of $p$ belong to $C_i$, the number of inner nodes of $p$ that belong to $A$ is at most $|A \cap C_i|$. Thus, we have,
	$$BS_i(A) \le |A \cap C_i|.$$
\end{proof}

\subsection{Proof of Theorem \ref{THEOREM:BC}}
\begin{proof}
	Recall from Lemma \ref{lemma:bcc}, $	bc(v) = {\gamma} \eta \risk_c^{(A)}(\sh_v) + bc_a(v)$.
	Thus, we have,
	\begin{align*}
	&\Pr \left[\forall v \in A, \tilde{bc}(v) - bc(v)| < \epsilon\right]\\
	=& \Pr \left[\forall v \in A,   \gamma \eta \erisk_v + bc_a(v)- ({\gamma} \eta \risk_c^{(A)}(\sh_v) + bc_a(v))| < \epsilon\right] \\
	=&\Pr\left[\forall v \in A, |\risk_c^{(A)}(\sh_v)-\erisk_v| < \epsilon^*\right]
	\end{align*}
	From line 8 in the algorithm, $\{\erisk_v\}_{v\in A}$ is obtained from \SSP{} framework. From Theorem \ref{LEMMA:SSP}, we have
	\begin{equation*}
	\Pr \left[\forall v \in A, |\risk_c^{(A)}(\sh_v)-\erisk_v| < \epsilon^*\right] \ge 1-\delta
	\end{equation*}
	This conclude our proof.
\end{proof}

\subsection{Proof of Lemma \ref{lemma:rt}}
\begin{proof}
	The time complexity to decompose a graph $G$  is $O(m+n)$.
	The time complexity to run \exactbc algorithm is $O(K)$ (see Lemma \ref{LEMMA:COMPLEXITY-subset}).
	The maximum number of sample is $O(\frac{1}{\epsilon^2}(\lfloor \log(BS(A)) \rfloor + 1+ln\frac{1}{\delta}))$. Plus, from Lemma \ref{lemma:samplecomp}, the time complexity to generate a sample is  $O(n^{1/2 + o(1)})$. Thus, in total, the time complexity of Algorithm~\ref{alg::RP} is  $O(m+n + K + \frac{1}{\epsilon^2}(\lfloor \log(BS(A)) \rfloor + 1+ln\frac{1}{\delta}) n^{1/2 + o(1)})$. 
\end{proof}
