# Supplementary material for: SaPHyRa: A Learning Theory Approach to Ranking Nodes in Large Networks
Source: arXiv:2203.01746 source file (2022-03-03)
Supplement: Supplementary file 2 [file Appendix.tex]

\begin{appendix}

We now readly to proof Theorem \ref{LEMMA:SSP}. 
\end{appendix}
